# Supplementary material for: TPMDP: Threshold Personalized Multi-party Differential Privacy via Optimal Gaussian Mechanism
Source: arXiv:2305.11192 source file (2023-05-30)
Supplement: Supplementary file 1 [file supplementary.tex]

%\hide{
\section{}
    \subsection{Proofs for Case 1: $*U = U$}\label{case1_proof}
    \begin{lemma}\label{lemma:DP_sort}
        For Case 1, if $\boldsymbol{\sigma}$ is feasible for Eq.~\eqref{eq:Gauss_opt}, then $\hat{\boldsymbol{\sigma}} \triangleq (\hat{\sigma}_i)_{i=1}^n$ is feasible, where $\hat{\boldsymbol{\sigma}}$ is a permutation of $\boldsymbol{\sigma}$ which satisfies $\hat{\sigma}_i^2 \geq \hat{\sigma}_j^2$ when {$\sigma_{\Gamma_i}$} $\geq$ {$\sigma_{\Gamma_j}$}.
    \end{lemma}
    \begin{proof}
        Without loss of generality, assume that {$\sigma_{\Gamma_j} \geq \sigma_{\Gamma_k}$} for $j<k$.
        Suppose, by contradiction, that $\hat{\boldsymbol{\sigma}}$ is not feasible for Eq.~\eqref{eq:Gauss_opt}, which implies that there exists $k\in \{1,\hdots,n\}$ such that Eq.~\eqref{eq:DP_min} does not hold. For $*U = U$, we have $*\mathcal{A}_\tau = \mathcal{A}_\tau$. As $\hat{\boldsymbol{\sigma}}$ is a permutation of $\boldsymbol{\sigma}$, it holds that $\{\min_{A_j} \Sigma_{i\in \bar{A}_j} \hat{\sigma}_i^2\}_{j=1}^n = \{\min_{A_j} \Sigma_{i\in \bar{A}_j} \sigma_i^2\}_{j=1}^n$, denoted by $E$. Then, it holds that $\min_{A_j} \Sigma_{i\in \bar{A}_j} \hat{\sigma}_i^2$ is the $j$-largest element in $E$. Because $\boldsymbol{\sigma}$ is feasible for Eq.~\eqref{eq:Gauss_opt}, it follows that for all $j\in \{1,\hdots,n\}$, $\min_{A_j} \Sigma_{i\in \bar{A}_j} \sigma_i^2 \geq \sigma_{\Gamma_j}^2$. It holds that $\min_{A_j} \Sigma_{i\in \bar{A}_j} \sigma_i^2 \geq$ {$ \sigma_{\Gamma_k}^2$} $ > \min_{A_k} \Sigma_{i\in \bar{A}_k} \hat{\sigma}_i^2$ for all $j\in \{1,\hdots,k\}$, 
        %Therefore, there are at least $k$ elements in $E$ strictly larger than $\min_{A_k} \Sigma_{i\in \bar{A}_k} \hat{\sigma}_i^2$, 
        which contradicts that $\min_{A_k} \Sigma_{i\in \bar{A}_k} \hat{\sigma}_i^2$ is the $k$-largest term in $E$.
    \end{proof}

    %Lemma \ref{lemma:DP_sort} states that we can restrict attention to those $\boldsymbol{\sigma}$'s satisfying $\sigma_i \geq \sigma_j$ when {$\sigma_{\Gamma_i}\geq \sigma_{\Gamma_j}$} as any feasible $\boldsymbol{\sigma}$ can be converted into a feasible $\hat{\boldsymbol{\sigma}}$ satisfying this requirement. This restriction is formalized in the following convention.
    %Formally, we formalize this idea in the following convention.
    
    By Lemma \ref{lemma:DP_sort}, we can restrict attention to those $\boldsymbol{\sigma}$'s satisfying the following convention as any feasible $\boldsymbol{\sigma}$ can be converted into a feasible $\hat{\boldsymbol{\sigma}}$ satisfying this convention.

    \begin{convention}\label{ass:Theta_sort_case1}
        $\boldsymbol{\sigma}$ satisfies that $\sigma_i^2 \geq \sigma_j^2$ when {$\sigma_{\Gamma_i}\geq \sigma_{\Gamma_j}$} for $i,j\in \{1,\hdots,n\}$.
    \end{convention}
    
    For simplifying notation, without loss in generality, we assume that $\sigma_{\Gamma_i}\ge \sigma_{\Gamma_j}$, $\forall i<j$ in the following lemmas in this subsection.
    
    \begin{lemma}\label{lemma:sort_iff_cond}
        For Case 1, let Convention \ref{ass:Theta_sort_case1} hold. Then $\boldsymbol{\sigma}$ is feasible for Eq.~\eqref{eq:Gauss_opt} if and only if for $j\leq \tau+1$,
        \begin{equation}\label{eq:sort_iff_cond}
            \sigma_j^2+\Sigma_{i=\tau+2}^n \sigma_i^2 \geq \sigma_{\Gamma_j}^2.
        \end{equation}
    \end{lemma}

    \begin{proof}
        ``$\Rightarrow$'' {It follows} from Lemma \ref{lemma:DP_min}.

        ``$\Leftarrow$'' By Convention \ref{ass:Theta_sort_case1}, it holds that $\min_{A_j} \Sigma_{i\in \bar{A}_j} \sigma_i^2 = \sigma_j^2+\Sigma_{i=\tau+2}^n \sigma_i^2 \geq \sigma_{\Gamma_j}^2$ for $j\leq \tau+1$. For $j \geq \tau+2$, we have $\min_{A_j} \Sigma_{i\in \bar{A}_j} \sigma_i^2 = \Sigma_{i=\tau+1}^n \sigma_i^2 \geq \sigma_{\Gamma_j}^2$. Thus, by Lemma \ref{lemma:DP_min}, $\boldsymbol{\sigma}$ is feasible for Eq.~\eqref{eq:Gauss_opt}.
    \end{proof}

    \begin{lemma}\label{lemma:3cond}
        For Case 1, let Convention \ref{ass:Theta_sort_case1} hold. If $\boldsymbol{\sigma}$ is optimal for Eq.~\eqref{eq:Gauss_opt}, then
        \begin{enumerate}
            \item $\sigma_{\tau+1}^2=\sigma_{\tau+2}^2=\hdots =\sigma_n^2$;
            \item for $j\leq \tau$, if $\sigma_j^2 > \sigma_{j+1}^2$, then $\sigma_j^2+\Sigma_{i=\tau+2}^n \sigma_i^2 = $ {$\sigma_{\Gamma_j}^2$};
            \item $\sigma_1^2+\Sigma_{i=\tau+2}^n \sigma_i^2 = $ {$\sigma_{\Gamma_1}^2$}.
        \end{enumerate}
    \end{lemma}
    \begin{proof}[Sketch of proof]
        1) Assume, by contradiction, that condition 1) does not hold. Construct $\hat{\boldsymbol{\sigma}}$ where $\hat{\sigma}_{\tau+2}^2=\frac{1}{n-\tau-1} \Sigma_{i=\tau+2}^n \sigma_i^2 + \gamma$, $\hat{\sigma}_i^2=\frac{1}{n-\tau-1} \Sigma_{i=\tau+2}^n \sigma_i^2$ for $i \geq \tau+3$ and $\hat{\sigma}_i^2=\sigma_i^2-\gamma$ for $i\leq \tau+1$, for some $\gamma$ sufficiently small. It holds that $\hat{\boldsymbol{\sigma}}$ is superior to $\boldsymbol{\sigma}$ for Eq.~\eqref{eq:Gauss_opt}, which constitutes a contradiction.

        2) Assume, by contradiction, that condition 2) does not hold for $\boldsymbol{\sigma}$ when $j = \xi$. Then, construct $\hat{\boldsymbol{\sigma}}$ as $\hat{\sigma}_\xi^2 = \sigma_\xi^2 - \gamma$ and $\hat{\sigma}_j^2 = \sigma_j^2$ for $j \neq \xi$, for $\gamma$ sufficiently small. It holds that $\hat{\boldsymbol{\sigma}}$ is superior to $\boldsymbol{\sigma}$ for Eq.~\eqref{eq:Gauss_opt}; contradiction.

        3) If there exists $j\leq n-1$ such that $\sigma_j^2 > \sigma_{j+1}^2$, then condition 3) holds from condition 1) and condition 2). {Otherwise}, suppose, by contradiction, that condition 3) does not hold. It holds that $\hat{\boldsymbol{\sigma}}$ is superior to $\boldsymbol{\sigma}$ where $\hat{\sigma}_i^2 = \frac{1}{n-\tau} \sigma_{\Gamma_1}^2$ for $i\in \{1,\hdots,n\}$; contradiction.
    \end{proof}

    \begin{lemma}\label{lemma:3cond_cor}
        For Case 1, let Convention \ref{ass:Theta_sort_case1} hold. There always exists an optimal $\boldsymbol{\sigma}$ for Eq.~\eqref{eq:Gauss_opt} such that there exists $\xi\leq \min{(\lfloor \frac{2n-\tau}{n-\tau} \rfloor, \tau+1)}$, $\sigma_{\xi}^2 = \sigma_{\xi+1}^2 = \hdots = \sigma_{n}^2$ and $\sigma_j^2+\Sigma_{i=\tau+2}^n \sigma_i^2 = \sigma_{\Gamma_j}^2$ for $j\leq \xi$.
    \end{lemma}

    \begin{proof}[Sketch of proof]
        For $\boldsymbol{\sigma}$ satisfying $\sigma_1^2 = \hdots = \sigma_n^2$, Lemma \ref{lemma:3cond_cor} holds from condition 3) in Lemma \ref{lemma:3cond} where $\xi = 1$. Otherwise, choose $\xi = \arg \max_j \sigma_{j-1}^2 > \sigma_{j}^2$. By condition 1) in Lemma \ref{lemma:3cond}, we have $\xi\leq \tau + 1$. It remains to prove $\sigma_j^2+\Sigma_{i=\tau+2}^n \sigma_i^2 = \sigma_{\Gamma_j}^2$ for $j\leq \xi$ and $\xi \leq \lfloor \frac{2n-\tau}{n-\tau} \rfloor$.

        For $j\leq \xi-1$, by Convention \ref{ass:Theta_sort_case1} and condition 2) in Lemma \ref{lemma:3cond}, it holds that $\sigma_j^2+\Sigma_{i=\tau+2}^n \sigma_i^2 = \sigma_{\Gamma_j}^2$. To prove $\xi \leq \lfloor \frac{2n-\tau}{n-\tau} \rfloor$, {suppose}, by contradiction, that $\xi > \lfloor \frac{2n-\tau}{n-\tau} \rfloor$. Construct $\hat{\boldsymbol{\sigma}}$ where $\hat{\sigma}_j^2 = \sigma_j^2 + \gamma$ for $j\geq \xi$ and $\hat{\sigma}_j^2 = \sigma_j^2 - (n-\tau-1)\gamma$ for $j\leq \xi-1$ with sufficiently small $\gamma$. {It holds that} $\hat{\boldsymbol{\sigma}}$ is superior to $\boldsymbol{\sigma}$ which yields a contradiction.

        Finally, if $\boldsymbol{\sigma}$ does not satisfy $\sigma_{\xi}^2+\Sigma_{i=\tau+2}^n \sigma_i^2 = \sigma_{\Gamma_{\xi}}^2$, construct $\hat{\boldsymbol{\sigma}}$ where $\hat{\sigma}_j^2 = \sigma_j^2 - \gamma$ for $j\geq \xi$ and $\hat{\sigma}_j^2 = \sigma_j^2 + (n-\tau-1)\gamma$ for $j\leq \xi-1$ with $\gamma = \sigma_{\xi}^2-\frac{1}{n-\tau} \sigma_{\Gamma_{\xi}}^2$. It holds that $\hat{\boldsymbol{\sigma}}$ is feasible and $v_{\hat{\boldsymbol{\sigma}}}\leq v_{\boldsymbol{\sigma}}$, which implies that there exists an optimal $\hat{\boldsymbol{\sigma}}$ for Eq.~\eqref{eq:Gauss_opt} satisfying Lemma \ref{lemma:3cond_cor}.
    \end{proof}

    \begin{proof}[Proof of Lemma \ref{lemma:exact_param}]\label{pf_lemma_exact_param}
        By Lemma \ref{lemma:3cond_cor}, $v_{\boldsymbol{\sigma}}$ corresponding to $\boldsymbol{\sigma}$ satisfying the requirement in Lemma \ref{lemma:3cond_cor} can be $\Sigma_{i=1}^{\xi-1} \sigma_{\Gamma_j}^2 + (\frac{2n-\tau}{n-\tau}-\xi) \sigma_{\Gamma_{\xi}}^2$ (denoted by $\mathcal{L}_\xi$) for $\xi\leq \min{(\lfloor \frac{2n-\tau}{n-\tau} \rfloor, \tau+1)}$. It holds that $\mathcal{L}_{\xi-1}-\mathcal{L}_{\xi} \geq 0$ for $\xi\leq \min{(\lfloor \frac{2n-\tau}{n-\tau} \rfloor, \tau+1)}$, which implies that $\boldsymbol{\sigma}$ in Lemma \ref{lemma:exact_param} is optimal.
        %Because $\boldsymbol{\sigma}_\xi=\mathcal{F}(\tau,n,\mathcal{E},\xi)$, by the definition of $\mathcal{F}$ we obtain that the value of the target function in Eq.~\eqref{eq:Gauss_opt} corresponding to $\boldsymbol{\sigma}_\xi$ is $\Sigma_{i=1}^{\xi-1} \sigma_{\Gamma_j}^2 + (\frac{2n-\tau}{n-\tau}-\xi)\sigma_{\Gamma_{\xi}}^2$, denoted by $\mathcal{L}_\xi$. We show that $\mathcal{L}_\xi \leq \mathcal{L}_j$ for $j\leq \tau+1$ when $\xi = \min{(\lfloor \frac{2n-\tau}{n-\tau} \rfloor, \tau+1)}$. Notice that $\mathcal{L}_{\xi-1} - \mathcal{L}_{\xi} = (\frac{2n-\tau}{n-\tau}-\xi)(\sigma_{\Gamma_{\xi-1}}^2-\sigma_{\Gamma_{\xi}}^2)$ for $\xi\in [2,\tau+1]$. Since $\sigma_{\Gamma_{\xi-1}}^2 \geq \sigma_{\Gamma_{\xi}}^2$ for $\xi\in [2,\tau+1]$, we have $\mathcal{L}_{\xi-1}-\mathcal{L}_{\xi} \geq 0$ for $\xi < \lfloor \frac{2n-\tau}{n-\tau} \rfloor$ and $\mathcal{L}_{\xi-1}-\mathcal{L}_{\xi} \leq 0$ for $\xi > \lfloor \frac{2n-\tau}{n-\tau} \rfloor$. Thus $\mathcal{L}_\xi \leq \mathcal{L}_j$ for $j\leq \tau$ when $\xi = \lfloor \frac{2n-\tau}{n-\tau} \rfloor$. So $\boldsymbol{\sigma}_\xi$ is optimal for Eq.~\eqref{eq:Gauss_opt} when $\xi = \min{(\lfloor \frac{2n-\tau}{n-\tau} \rfloor,\tau+1)}$.
    \end{proof}
    
    \begin{proof}[Proof of Lemma \ref{lemma:trivial_case}]\label{pf_lemma_trivial_case}
        By Eq.~\eqref{eq:DP_multi_Gaussian}, $\boldsymbol{\sigma}$ is feasible if and only if $\sigma_i^2 \geq \sigma_{\Gamma_i}^2,\, i\in U$ for $\tau = n-1$. Thus $(\sigma_{\Gamma_i})_{i=1}^n$ is optimal.
    \end{proof}

    \begin{proof}[Proof of Theorem \ref{thm:case_trivial}]
        %By Lemma \ref{lemma:exact_param} and Lemma \ref{lemma:trivial_case}, it is not difficult to verify that the solution computed by Alg. \ref{alg:DP_OPS_trivial} is optimal for Eq.~\eqref{eq:Gauss_opt} when $*U=U$.
        %
        %To prove the solution computed by Alg. \ref{alg:DP_OPS_trivial} is optimal for Eq.~\eqref{eq:Gauss_opt}, we show that $\hat{\boldsymbol{\sigma}} = \{\hat{\sigma}_i\}_{i\in U}$ is consistent with the results from Lemma \ref{lemma:exact_param} and Lemma \ref{lemma:trivial_case} where $\hat{\sigma}_i$ is computed by Alg. \ref{alg:DP_OPS_trivial} with parameters $F$, $(\tau,n,\mathcal{E})$ and $i$ for $i\in U$.
        %
        For $\tau = n-1$, it holds that Lines $1$--$3$ in Alg. \ref{alg:DP_OPS_trivial} produce the same $\sigma_i^2$ as the one in Lemma \ref{lemma:trivial_case}, which implies $\boldsymbol{\sigma} = (\sigma_i)_{i=1}^n$ is optimal. As $\sigma_{\Gamma_i}$ can be obtained in $\mathcal{O}(1)$ steps, the complexity of Alg. \ref{alg:DP_OPS_trivial} for $\tau = n-1$ is $\mathcal{O}(1)$.
    
        %First, it is trivial to verify that Line $1$ to Line $3$ in Alg. \ref{alg:DP_OPS_trivial} present the optimal solution in case $\tau = n-1$ by Lemma \ref{lemma:trivial_case}.
    
        For $\tau \leq n-2$, $\sigma_i^2$ computed from Lines $5$--$8$ in Alg. \ref{alg:DP_OPS_trivial} is the same as the one in Lemma \ref{lemma:trivial_case}, so $\boldsymbol{\sigma} = (\sigma_i)_{i=1}^n$ is optimal. As the complexity of Lines $5$, $6$, $8$ is $\mathcal{O}(1)$ and complexity of Line 7 is $\mathcal{O}(n)$, the total complexity of Alg. \ref{alg:DP_OPS_trivial} is $\mathcal{O}(n)$.
    \end{proof}

    \subsection{Proofs in Case 2: $*U\subset U$}

    \begin{proof}[Proof of Lemma \ref{lemma:DP_active_equiv}]
        Using \emph{Pigeonhole Principle}, the $\mathcal{U}_j$ defined in Corollary \ref{cor:DP_min2} is exactly the same for $j\in U$ when the active set is $*U$ or $U$. Thus by Corollary \ref{cor:DP_min2}, the feasible solutions for Eq.~\eqref{eq:Gauss_opt} in both cases coincide.
    \end{proof}

    \begin{proof}[Proof of Lemma \ref{lemma:*U_1_trivial}]
        First, we show that $\sigma_{1^*}^2 = 0$. Assume, by contradiction, that $\sigma_{1^*}^2 > 0$. Construct $\hat{\boldsymbol{\sigma}}$ such that $\hat{\sigma}_{1^*}^2 = 0$ and $\hat{\sigma}_j^2 = \sigma_j^2$ for $j\neq 1^*$. Then $\hat{\boldsymbol{\sigma}}$ is superior to $\boldsymbol{\sigma}$; contradiction.

        For $\tau \geq 2$, as we have proved that $\sigma_{1^*}^2 = 0$, we only need to show that Eq.~\eqref{eq:Gauss_opt} with parameter $(\tau,n,\mathcal{E})$ and $\left | *U \right | = 1$ is equivalent to Eq.~\eqref{eq:Gauss_opt} with parameter $(\tau-1,n-1,\overline{*\mathcal{E}}\})$ and active set $\overline{*U}$ when taking $\sigma_{1^*}^2 = 0$. As the objective function of Eq.~\eqref{eq:Gauss_opt} in these two cases are equivalent when $\sigma_{1^*}^2 = 0$, we only have to prove that the feasible solutions for these two problems coincide. As $1^*$ is the only active party in $U$, it holds that $\{\bar{A} | A\in *\mathcal{A}_\tau\}$'s are the same in these two cases. By Eq.~\eqref{eq:DP_multi_Gaussian}, the feasible solutions for these two problems are identical.

        For $\tau = 1$, $\mathcal{A}_\tau$ contains exactly only one element, i.e., $\{1^*\}$. Thus, $\boldsymbol{\sigma}$ is feasible for Eq.~\eqref{eq:Gauss_opt} if and only if $\Sigma_{i=1}^{n-1} \sigma_i^2 \geq \max_{j \in \overline{*U}} \sigma_{\Gamma_j}^2$. So $\Sigma_{i=1}^{n-1} \sigma_i^2 = \max_{j \in \overline{*U}} \sigma_{\Gamma_j}^2$ is optimal.
    \end{proof}

    The next lemma shows that a specific permutation of a feasible $\boldsymbol{\sigma}$ is also feasible. We omit the proof for length considerations. The proof is similar to that of Lemma \ref{lemma:DP_sort}, the main difference being that we need to evaluate the permutations of $*\boldsymbol{\sigma}$ and $\overline{*\boldsymbol{\sigma}}$ separately.

    \begin{lemma}\label{lemma:DP_sort_active}
        If $\boldsymbol{\sigma}$ is feasible for Eq.~\eqref{eq:Gauss_opt}, then ${\boldsymbol{\sigma}}' \triangleq ({\sigma}_i')_{i\in U}$ is feasible for Eq.~\eqref{eq:Gauss_opt}, where ${*\boldsymbol{\sigma}'}$ is a permutation of $*\boldsymbol{\sigma}$ which satisfies ${{\sigma}_{i^*}'}^2 \geq {{\sigma}_{j^*}'}^2$ when $\sigma_{\Gamma_{i^*}} \geq \sigma_{\Gamma_{j^*}}$ and ${\overline{*\boldsymbol{\sigma}'}}$ is a permutation of $\overline{*\boldsymbol{\sigma}}$ which satisfies ${{\sigma}_{i}'}^2 \geq {{\sigma}_{j}'}^2$ when $\sigma_{\Gamma_{i}} \geq \sigma_{\Gamma_{j}}$.
    \end{lemma}

    By Lemma \ref{lemma:DP_sort_active}, we can conclude that we can restrict attention to $\boldsymbol{\sigma}$'s satisfying the following convention.

    \begin{convention}\label{ass:Theta_sort_case2}
        $\boldsymbol{\sigma}$ satisfies that $\sigma_{{i}}^2 \geq \sigma_{{j}}^2$ when $\sigma_{\Gamma_{i}} \geq \sigma_{\Gamma_{j}}$ and $\sigma_{{i^*}}^2 \geq \sigma_{{j^*}}^2$ when $\sigma_{\Gamma_{i^*}} \geq \sigma_{\Gamma_{j^*}}$.
    \end{convention}
    
    Similarly as in Case $1$, we assume that $\sigma_{\Gamma_{i}} \geq \sigma_{\Gamma_{j}}$, $\forall i<j$ and $\sigma_{\Gamma_{i^*}} \geq \sigma_{\Gamma_{j^*}}$, $\forall i<j$ in the following lemmas without loss in generality.

    \begin{lemma}\label{lemma:2*_trivial}
        Let Convention \ref{ass:Theta_sort_case2} hold and $2 \leq \left| *U \right| \leq n-\tau$. If $\boldsymbol{\sigma}$ is optimal for Eq.~\eqref{eq:Gauss_opt} and $\sigma_{2^*}^2 \geq \sigma_{\tau}^2$, then $\hat{\boldsymbol{\sigma}}$ which is optimal for Eq.~\eqref{eq:Gauss_opt} with active set $U$ is optimal for Eq.~\eqref{eq:Gauss_opt} with active set $*U$.
    \end{lemma}

    \begin{proof}[Sketch of proof]
        By Lemma \ref{lemma:DP_min}, {one can verify} that $\boldsymbol{\sigma}$ is feasible for Eq.~\eqref{eq:Gauss_opt} when replacing $*U$ by $U$. As $*\mathcal{A}_\tau \subset \mathcal{A}_\tau$, it holds that all feasible solutions for Eq.~\eqref{eq:Gauss_opt} with active set $U$ is also feasible for Eq.~\eqref{eq:Gauss_opt} with active set $*U$. Thus, $\hat{\boldsymbol{\sigma}}$ is optimal for Eq.~\eqref{eq:Gauss_opt} with active set $*U$.
    \end{proof}

    By Lemma \ref{lemma:2*_trivial}, $\boldsymbol{\sigma}$ satisfying $\sigma_{2^*}^2\geq \sigma_{\tau}^2$ under Convention \ref{ass:Theta_sort_case2} is not superior to that obtained from Alg. \ref{alg:DP_OPS_trivial}. Thus, we restrict attention to a special class of $\boldsymbol{\sigma}$'s specified in the following convention.

    \begin{convention}\label{ass:2*_tau_cmp}
        Let $2 \leq \left| *U \right| \leq n-\tau$, $\boldsymbol{\sigma}$ satisfies $\sigma_{2^*}^2\leq \sigma_{\tau}^2$.
    \end{convention}

    \begin{lemma}\label{lemma:sort_iff_cond_active}
        Let Convention \ref{ass:2*_tau_cmp} hold. Then $\boldsymbol{\sigma}$ is feasible for Eq.~\eqref{eq:Gauss_opt} if and only if
        \begin{equation}\label{eq:sort_iff_cond_active}
        \left\{
        \begin{aligned}
            &\sigma_j^2+\Sigma_{i\in E} \sigma_i^2 \geq \sigma_{\Gamma_j}^2,\, j\in \{1,\hdots,\tau\} \\
            &\sigma_{\tau}^2+\Sigma_{i\in E} \sigma_i^2 \geq \sigma_{\Gamma_{2^*}}^2 \\
            &\sigma_{1^*}^2+\Sigma_{i\in E} \sigma_i^2-\sigma_{2^*}^2+\sigma_{\tau}^2 \geq \sigma_{\Gamma_{1^*}}^2,
        \end{aligned}
        \right.
        \end{equation}
        where $E=\{2^*,\hdots,(\eta+1)^*, \tau+1, \hdots, n-\eta-1\}$.
    \end{lemma}
    \begin{proof}[Sketch of proof]
        Eq.~\eqref{eq:sort_iff_cond_active} is equivalent to Eq.~\eqref{eq:DP_min} under Convention \ref{ass:2*_tau_cmp}.
    \end{proof}

    \begin{lemma}\label{lemma:DP_2cond_active}
        %Given an active set $*U$, the query function $F$ and the parameter $(\tau,n,\mathcal{E})$ where $2 \leq \left| *U \right| \leq n-\tau$ and $\mathcal{E}$ satisfies $\sigma_{\Gamma_{i}} \geq \sigma_{\Gamma_{j}}$, $\forall i<j$ and $\sigma_{\Gamma_{i^*}} \geq \sigma_{\Gamma_{j^*}}$, $\forall i<j$, then a ``sorted'' $\boldsymbol{\sigma}$ which satisfies Eq.~\eqref{eq:sort_iff_cond_active_cond} satisfies the requirement of $(\tau,n,\mathcal{E})$-TPMDP

        Let Convention \ref{ass:2*_tau_cmp} hold. Then $\boldsymbol{\sigma}$ is feasible for Eq.~\eqref{eq:Gauss_opt} if and only if $\boldsymbol{\sigma}$ is feasible when replacing $(\sigma_{\Gamma_i})_{i\in U}$ by $(\tilde{\sigma}_{\Gamma_i})_{i\in U}$ where
        \begin{equation}\label{eq:sort_iff_cond_active4}
            \left\{
            \begin{aligned}
                &\tilde{\sigma}_{{\Gamma}_{i}} = \max\{ \sigma_{\Gamma_{i}}, \sigma_{\Gamma_{2^*}}\},\, i\in \{1,\hdots,\tau\} \\
                &\tilde{\sigma}_{{\Gamma}_{j}}=\sigma_{\Gamma_j},\, \text{otherwise}.
            \end{aligned}
            \right.
        \end{equation}
    \end{lemma}
    \begin{proof}
        It follows from Lemma \ref{lemma:sort_iff_cond_active}.
    \end{proof}

    With Lemma \ref{lemma:DP_2cond_active}, we can restrict attention to a special class of $(\sigma_{\Gamma_i})_{i\in U}$ under Convention \ref{ass:2*_tau_cmp}, which is given in the following convention.

    \begin{convention}\label{ass:tau_2*_max_cond}
        Let Convention \ref{ass:2*_tau_cmp} hold, it holds that
        $$
            \sigma_{\Gamma_j}\geq \sigma_{\Gamma_{2^*}},\, \text{for }i\in \{1,\hdots,\tau\}.
        $$
    \end{convention}

    A direct corollary of Lemma \ref{lemma:sort_iff_cond_active} under Convention \ref{ass:tau_2*_max_cond} follows.

    \begin{corollary}\label{cor:sort_iff_cond_cor_active}
        Let Convention \ref{ass:tau_2*_max_cond} hold. Then $\boldsymbol{\sigma}$ is feasible for Eq.~\eqref{eq:Gauss_opt} if and only if
        \begin{equation}\label{eq:sort_iff_cond_cor_active}
        \left\{
        \begin{aligned}
            &\sigma_j^2+\Sigma_{i\in E} \sigma_i^2 \geq \sigma_{\Gamma_j}^2,\, \text{for }j\in \{1,\hdots,\tau\} \\
            &\sigma_{1^*}^2+\Sigma_{i\in E} \sigma_i^2-\sigma_{2^*}^2+\sigma_{\tau}^2 \geq \sigma_{\Gamma_{1^*}}^2.
        \end{aligned}
        \right.
        \end{equation}
    \end{corollary}

    In the following lemma, we present several necessary conditions for the optimal solutions of Eq.~\eqref{eq:Gauss_opt} under Convention \ref{ass:tau_2*_max_cond}. We omit the proof for length considerations. The proof is similar to that of the first two conditions in Lemma \ref{lemma:3cond}, the main difference being that here we invoke the feasibility condition provided by Corollary \ref{cor:sort_iff_cond_cor_active}.

    \begin{lemma}\label{lemma:DP_3cond_active}
        Let Convention \ref{ass:tau_2*_max_cond} hold. If $\boldsymbol{\sigma}$ is optimal for Eq.~\eqref{eq:Gauss_opt}, then
        \begin{enumerate}
            \item if $\tau\geq 2$, $\sigma_{\tau}^2=\sigma_{\tau+1}^2=\hdots =\sigma_{n-\eta-1}^2$;
            \item $\sigma_{2^*}^2=\sigma_{3^*}^2=\hdots=\sigma_{(\eta+1)^*}^2$;
            \item for $j\leq \tau-1$, if $\sigma_j^2 > \sigma_{j+1}^2$, then $\sigma_j^2+\Sigma_{i\in E} \sigma_i^2  = \sigma_{\Gamma_j}^2$.
        \end{enumerate}
    \end{lemma}

    \begin{lemma}\label{lemma:DP_6cond_active}
        %Given an active set $*U$, the query function $F$ and the parameter $(\tau,n,\mathcal{E})$ where $2 \leq \left| *U \right| \leq n-\tau$ and $\mathcal{E}$ satisfies Eq.~\eqref{eq:tau_2*_max_cond} and $\sigma_{\Gamma_{i}} \geq \sigma_{\Gamma_{j}}$, $\forall i<j$ and $\sigma_{\Gamma_{i^*}} \geq \sigma_{\Gamma_{j^*}}$, $\forall i<j$, if a ``sorted'' $\boldsymbol{\sigma}$ satisfies Eq.~\eqref{eq:sort_iff_cond_active_cond} and is optimal for Eq.~\eqref{eq:Gauss_opt},

        Let Convention \ref{ass:tau_2*_max_cond} hold. If $\boldsymbol{\sigma}$ is optimal for Eq.~\eqref{eq:Gauss_opt}, then
        \begin{enumerate}
            \item if $n-\tau-\tau\eta\leq 0$, $\boldsymbol{\sigma}$ is not superior to the optimal solution of Eq.~\eqref{eq:Gauss_opt} with active set $U$;
            \item if $n-\tau-\tau\eta> 0$, $\sigma_{2^*}^2=0$.
        \end{enumerate}
    \end{lemma}
    \begin{proof}
        For $n-\tau-\tau\eta \leq 0$, by Lemma \ref{lemma:2*_trivial}, we only need to prove that there exists an optimal $\boldsymbol{\sigma}$ under Convention \ref{ass:tau_2*_max_cond} satisfying $\sigma_{2^*}^2 = \sigma_{\tau}^2$. If $\boldsymbol{\sigma}$ does not satisfy $\sigma_{2^*}^2 = \sigma_{\tau}^2$, construct $\hat{\boldsymbol{\sigma}}$ as $\hat{\sigma}_{j}^2 = \sigma_{j}^2 + \gamma$ for $j \in *U$ and $\hat{\sigma}_j^2 = \sigma_j^2-\frac{\eta}{n-\eta-\tau}\gamma$ for $j \in \overline{*U}$ where $\gamma = \frac{2n-\eta-\tau}{n-\eta-\tau} (\sigma_{\tau}^2 - \sigma_{2^*}^2)$. It holds that $\hat{\boldsymbol{\sigma}}$ satisfies $\sigma_{2^*}^2 = \sigma_{\tau}^2$ and is not inferior to $\boldsymbol{\sigma}$ for Eq.~\eqref{eq:Gauss_opt}.

        For $n-\tau-\tau\eta > 0$, assume, by contradiction, that $\boldsymbol{\sigma}$ does not satisfy $\sigma_{2^*}^2 = 0$. Construct $\hat{\boldsymbol{\sigma}}$ as $\hat{\sigma}_{j}^2 = \sigma_{j}^2 - \gamma$ for $j \in *U$ and $\hat{\sigma}_j^2 = \sigma_j^2+\frac{\eta}{n-\eta-\tau}\gamma$ for $j \in \{1,\hdots, n-\eta-1\}$ with a sufficiently small $\gamma$. Consequently, $\hat{\boldsymbol{\sigma}}$ is superior to $\boldsymbol{\sigma}$ for Eq.~\eqref{eq:Gauss_opt} under Convention \ref{ass:tau_2*_max_cond}, a contradiction.
    \end{proof}

    \begin{proof}[Proof of Lemma \ref{lemma:DP_6cond_active_cor}]
    {It follows} from Lemma \ref{lemma:DP_6cond_active} \& \ref{lemma:2*_trivial}.
    \end{proof}

    \begin{proof}[Proof of Lemma \ref{lemma:tau_1_case_active}]
        As $\boldsymbol{\sigma}$ satisfies Convention \ref{ass:2*_tau_cmp}, it holds that $\boldsymbol{\sigma}$ is feasible for Eq.~\eqref{eq:Gauss_opt} by Eq.~\eqref{eq:sort_iff_cond_active}. Assume, by contradiction, that $\boldsymbol{\sigma}$ is not optimal, then there exists $\hat{\boldsymbol{\sigma}}$ superior to $\boldsymbol{\sigma}$. Notice that $\boldsymbol{\sigma}$ satisfies $\Sigma_{i\in U} \sigma_i^2 = \max \{\sigma_{\Gamma_{1^*}}^2, \sigma_{\Gamma_{1}}^2, \sigma_{\Gamma_{2^*}}^2\}$ while it holds that $\Sigma_{i\in U} \hat{\sigma}_i^2 \geq \max_{i\in U} \sigma_{\Gamma_{i}}^2 \geq \max \{\sigma_{\Gamma_{1^*}}^2, \sigma_{\Gamma_{1}}^2,$ $ \sigma_{\Gamma_{2^*}}^2\}$. Thus, we have $\Sigma_{i\in U} \hat{\sigma}_i^2 \geq \Sigma_{i\in U} \sigma_i^2$; contradiction.
    \end{proof}

    For Subcase \ref{subcase_5}, we present three necessary conditions for $\boldsymbol{\sigma}$ to be optimal for Eq.~\eqref{eq:Gauss_opt} under Convention \ref{ass:tau_2*_max_cond} in Lemma \ref{lemma:DP_5cond_active}. We omit the details for length considerations. The proof for the first condition is similar to that for condition 3) in Lemma \ref{lemma:3cond} and proofs for the other two conditions are similar to that of Lemma \ref{lemma:3cond_cor}.

    \begin{lemma}\label{lemma:DP_5cond_active}
        For Subcase \ref{subcase_5}, let Convention \ref{ass:tau_2*_max_cond} hold. If $\boldsymbol{\sigma}$ is optimal for Eq.~\eqref{eq:Gauss_opt}, then
        \begin{enumerate}
            \item $\sigma_1^2+\Sigma_{i\in E} \sigma_i^2  = \sigma_{\Gamma_1}^2$;
            \item there exists $1\leq \xi \leq \tau$ such that $\sigma_{\xi}^2 = \sigma_{\xi + 1}^2=\hdots=\sigma_{n-\eta-1}^2$, and $ \sigma_{j}^2+\Sigma_{i\in E} \sigma_i^2 =\sigma_{\Gamma_{j}}^2, \forall j \leq \xi-1$;
            \item $\xi$ as defined in condition 2) satisfies $\xi=1$ if $\sigma_{1^*}^2>0$ and $\xi\leq 2$ if $\sigma_{1^*}^2=0$.
        \end{enumerate}

    \end{lemma}

    \begin{proof}[Proof of Lemma \ref{lemma:nontrivial_noise_active} (sketch)]
        For condition 1), assume, by contradiction, that there does not exist an optimal solution satisfying Convention \ref{ass:2*_tau_cmp}. By Lemma \ref{lemma:2*_trivial}, it holds that $\boldsymbol{\sigma}$ is strictly inferior to the solution obtained from Alg. \ref{alg:DP_OPS_trivial}. On the other hand, we can reason that $\boldsymbol{\sigma}$ is no worse than the solution obtained from Alg. \ref{alg:DP_OPS_trivial} via a simple algebraic computation, which yields a contradiction. Subsequently, by Lemma \ref{lemma:DP_2cond_active}, we can transform Eq.~\eqref{eq:Gauss_opt} %in this case
        into an equivalent problem by replacing $(\sigma_{\Gamma_i})_{i\in U}$ with $(\tilde{\sigma}_{\Gamma_i})_{i\in U}$ as defined in Lemma \ref{lemma:DP_2cond_active}. It holds that $\boldsymbol{\sigma}$ in condition 1) satisfies the necessary conditions in Lemma \ref{lemma:DP_5cond_active} with $\xi = 1$. We can further show that $\boldsymbol{\sigma}$ is optimal when $\xi = 1$. By condition 3) in Lemma \ref{lemma:DP_5cond_active}, we have that $\xi$ can only take value $1$ or $2$; additionally, it follows from the same lemma that the value for $\xi=1$ is strictly smaller than for $\xi=2$.
        %Thus, by comparing $\boldsymbol{\sigma}$ with the optimal one specified in
        %Lemma \ref{lemma:DP_5cond_active} when $\xi = 2$, we prove that $\boldsymbol{\sigma}$ in condition 1) is optimal for Eq.~\eqref{eq:Gauss_opt}.
        For condition 2), the proof follows similar arguments.
    \end{proof}

    \begin{proof}[Proof of Theorem \ref{thm:case_general_rst} (sketch)]
        $\ \ $\\
        \textbf{Optimality}:
        \begin{itemize}
            \item Lines $1$--$9$ in Alg. \ref{alg:DP_OPS_2} generate the optimal $\sigma_i,\ i\in U$  following Lemma \ref{lemma:*U_1_trivial};
            \item Lines $10$--$12$ follow Lemma \ref{lemma:DP_active_equiv} and Lemma \ref{lemma:DP_6cond_active_cor};
            \item Lines $13$--$24$ follow Lemma \ref{lemma:tau_1_case_active};
            \item Lines $25$--$38$ follow Lemma \ref{lemma:nontrivial_noise_active}.
        \end{itemize}
    
        \noindent \textbf{Complexity}:
        \begin{itemize}
            \item if $\tau = n-1$, the complexity is $\mathcal{O}(1)$ for Lines $1$--$9$ \& $10$--$12$;
            \item if $\left| *U \right| =1$ and $i\in *U$, the complexity is $\mathcal{O}(1)$ for Lines $2$--$3$;
            \item otherwise, Alg. \ref{alg:DP_OPS_2} needs to compute $\sigma_{\Gamma_j}$ for $j\in U$ and find the largest and $2$-largest elements in $(\sigma_{\Gamma_j})_{j\in *U}$ and $(\sigma_{\Gamma_j})_{j\in \overline{*U}}$ (i.e., Lines $13$--$17$), whose complexity is $\mathcal{O}(n)$.
        \end{itemize}%
    \end{proof}
%}

\hide{

\section{Proof in Section \ref{sec:perform}}\label{app:perform}
    \begin{proof}[Proof of Theorem \ref{thm:v_G_lo} (sketch)]
        For Subcase \ref{subcase_1}, as it degenerates to Case 1, we only need to consider $*U = U$. Without loss of generality, assume that $\sigma_{\Gamma_i}\ge \sigma_{\Gamma_j}$, $\forall i<j$. %It holds that when $n > 2\tau$, $\xi$ in Alg. \ref{alg:DP_OPS_trivial} equals to $2$. 
        For Setting \ref{setting_1}, by Alg. \ref{alg:DP_OPS_trivial}, $v_{G} = \sigma_{\Gamma_1}^2 + \frac{\tau}{n-\tau} \sigma_{\Gamma_2}^2$ when $n>2\tau$. As it holds that $v_{MIN} = \sigma_{\Gamma_1}^2$, it follows that: $\frac{v_G}{v_{MIN}} \leq 1+\frac{\tau}{n-\tau} = \mathcal{O}(1).$
        For Setting \ref{setting_2}, when $n>\frac{1}{p(1-p)}$, it holds that $v_{G} = \Sigma_{i=1}^{\xi-1} \sigma_{\Gamma_i}^2 + (\frac{2n-\tau}{n-\tau} - \xi) \sigma_{\Gamma_{\xi}}^2$ where $\xi = \lfloor 2 + \frac{p}{1-p} \rfloor$, which implies $\frac{v_G}{v_{MIN}} = \mathcal{O}(1)$.
        The proofs for Subcases $\ref{subcase_2}-\ref{subcase_5}$ are similar.
    \end{proof}

    \begin{proof}[Proof of Theorem \ref{thm:v_up_O}]
        Similar to the proof for Theorem \ref{thm:v_G_lo}.
    \end{proof}
}

%\hide{
\subsection{Composition Properties of TPMDP}\label{app:comp}
      
    Similar to the composition theorems in DP \cite{dwork2014algorithmic}, TPMDP also features composition properties. 
    Formally, if multiple TPMDP mechanisms execute independently on a common input 
    $\bar{x}$, the composed mechanism also satisfies a TPMDP requirement. 
    In this appendix, we present the composition properties for TPMDP.
    First, we formalize the setting of composition theorems in the following assumption.
    
    \begin{assumption}\label{ass:comp_mech}
        $\Pi^{(j)}$ is a $(\tau,n,\mathcal{E}^{(j)})$-TPMDP mechanism with input $\bar{x}$ for $j\in \{1,\hdots,m\}$ where $\mathcal{E}^{(j)}\triangleq ((\epsilon^{(j)}_i, \delta^{(j)}_i))_{i=1}^n$ and $\Pi^{(j)},\, j\in \{1,\hdots,m\}$ are mutually independent. The refined view for $A\in \mathcal{A}_\tau$ in $\Pi^{(j)}$ is $\mathcal{RV}_A^{\Pi^{(j)}}(\bar{x},\bar{X}^{(j)})$ for $j\in \{1,\hdots,m\}$. The composed mechanism $(\Pi^{(1)}, \hdots, \Pi^{(m)})$ is denoted as $\Pi$.
    \end{assumption}
    
    To prove the composition theorems for TPMDP, we first establish a lemma which gives a refined view for the composed mechanism $\Pi$ in Assumption~\ref{ass:comp_mech}.
    
    %Before presenting this lemma, we first make an important convention that all
    
    %Now we would give the lemma presenting the refined view for composed mechanisms.
    
    \begin{lemma}\label{lemma:RV_comb}
        Let Assumption \ref{ass:comp_mech} hold. For $A\in \mathcal{A}_\tau$, the composed refined view $(\mathcal{RV}_A^{\Pi^{(j)}}(\bar{x},\bar{X}^{(j)}))_{j=1}^m$ is
        \begin{enumerate}
            \item a perfect refined view for $\Pi$ if $\mathcal{RV}_A^{\Pi^{(j)}}(\bar{x},\bar{X}^{(j)})$ is a perfect refined view in $\Pi^{(j)}$ for $j\in \{1,\hdots,m\}$;
            \item a statistical (computational) refined view for $\Pi$ if $\mathcal{RV}_A^{\Pi^{(j)}}(\bar{x},\bar{X}^{(j)})$ is a statistical (computational) refined view in $\Pi^{(j)}$ for $j\in \{1,\hdots,m\}$ and $m$ is polynomial related to $\left| \bar{x}\right|$.
        \end{enumerate}
    \end{lemma}
    
    Before presenting the proof, we first present an assumption.

    \begin{assumption}\label{ass:comp_en}
        Given are two collections of mutually independent ensembles $\{X^{(j)}\}_{j=1}^m$ and $\{X^{(j)}\}_{j=1}^m$, where 
        also $\{X^{(1)}, \hdots, X^{(i)}, Y^{(i+1)}, \hdots, Y^{(m)}\}$ are mutually independent collections, for each $i=1,\hdots,m-1$. Define the composed ensembles $\{(X_w^{(1)}, \hdots, X_w^{(m)})\}_{w\in E}$ and $\{(Y_w^{(1)}, \hdots, Y_w^{(m)})\}_{w\in E}$ to be $X$ and $Y$ respectively.
    \end{assumption}

    \begin{lemma}\label{lemma:comp_en}
        Let Assumption \ref{ass:comp_en} hold. Then
        \begin{enumerate}
            \item $X$ and $Y$ are perfectly indistinguishable if $X^{(i)}$ and $Y^{(i)}$ are perfectly indistinguishable for $i\in \{1,\hdots,m\}$;
            \item $X$ and $Y$ are computationally (statistically) indistinguishable if $X^{(i)}$ and $Y^{(i)}$ are computationally (statistically) indistinguishability for $i\in \{1,\hdots,m\}$ and $m$ is polynomial related to $\left| w \right|$.
        \end{enumerate}
    \end{lemma}
    \begin{proof}[Sketch of proof]
        For perfect and statistical indistinguishability, Lemma \ref{lemma:comp_en} can be proved by evaluating the LHS of Eq.~\eqref{eq:s_ind}. For computational indistinguishability, Lemma \ref{lemma:comp_en} can be proved using the \emph{hybrid technique}~\cite{goldreich2007foundations}.
    \end{proof}

    \begin{proof}[Proof of Lemma \ref{lemma:RV_comb}]
        For the perfect refined view, by Assumption \ref{ass:comp_mech}, $\{\mathcal{V}_A^\Pi (\bar{x},\bar{X}^{(j)})\}_{\bar{x}\in (\{0,1\}^{*})^n,\bar{X}^{(j)}\in \mathcal{P}^n}$ and $\{\mathcal{S}^{(j)}(A, \mathcal{RV}_A^\Pi (\bar{x},\bar{X}^{(j)}))\}_{\bar{x}\in (\{0,1\}^{*})^n,\bar{X}^{(j)}\in \mathcal{P}^n}$, $j \in \{1, \hdots, m\}$ satisfy Assumption \ref{ass:comp_en} where $\mathcal{S}^{(j)}$ is defined as in Definition \ref{def:rView}. By Lemma \ref{lemma:comp_en}, 
        %we have
        %$$
        %    \begin{aligned}
        %        \{(\mathcal{S}^{(j)}(A, & \mathcal{RV}_A^\Pi (\bar{x},\bar{X}^{(j)})))_{j=1}^m\}_{\bar{x}\in (\{0,1\}^{*})^n,\bar{X}^{(j)}\in \mathcal{P}^n} \overset{perf}\equiv \\
        %        &\qquad \{(\mathcal{V}_A^\Pi (\bar{x},\bar{X}^{(j)}))_{j=1}^m\}_{\bar{x}\in (\{0,1\}^{*})^n,\bar{X}^{(j)}\in \mathcal{P}^n}
        %    \end{aligned}
        %$$
        %Consequently, 
        $(\mathcal{RV}_A^{\Pi^{(j)}}(\bar{x},\bar{X}^{(j)}))_{j=1}^m$ is a refined view for $\Pi$. For statistical and computational refined views, the proofs are similar.
    \end{proof}
    %}
    
    Now we present the composition theorems for TPMDP, Theorems \ref{thm:m_comp_thm} and \ref{thm:m_A_comp}. We omit the proof of Theorem \ref{thm:m_A_comp}, which is similar to that of Theorem \ref{thm:m_comp_thm}, the main difference being that in Theorem \ref{thm:m_A_comp} the advanced composition of DP \cite{dwork2014algorithmic} is used.
    
    %We will first consider a general case where $n$ parites independently execute $m$ $(\tau,n,\mathcal{E}^{(i)})$-TPMDP mechanisms with input $\bar{x}$, where $i\in \{1,\hdots,m\}$.
    
    \begin{theorem}[Composition for TPMDP] \label{thm:m_comp_thm}
        Let Assumption \ref{ass:comp_mech} hold and $\mathcal{E} = ((\Sigma_{j=1}^m \epsilon_i^{(j)}, \Sigma_{j=1}^m \delta_i^{(j)}))_{i=1}^n$. Then $\Pi$ is
        \begin{enumerate}
            \item perfectly $(\tau,n,\mathcal{E})$-TPMDP if $\Pi^{(j)}$ is perfectly $(\tau,n,\mathcal{E}^{(j)})$-TPMDP for $j\in \{1,\hdots,m\}$;
            \item statistically (computationally) $(\tau,n,\mathcal{E})$-TPMDP if $\Pi^{(j)}$ is statistically (computationally) $(\tau,n,\mathcal{E}^{(j)})$-TPMDP for $j\in \{1,\hdots,m\}$ and $m$ is polynomial related to $\left| \bar{x} \right|$.
        \end{enumerate}
    %    where $\mathcal{E} = ((\Sigma_{j=1}^m \epsilon_i^{(j)}, \Sigma_{j=1}^m \delta_i^{(j)}))_{i=1}^n$.
    \end{theorem}
    
    \begin{proof}
        For perfectly TPMDP, since $\Pi^{(j)}$ is perfectly $(\tau,n,\mathcal{E}^{(j)})$-TPMDP for $j\in \{1,\hdots,m\}$, by Eq.~\eqref{eq:tMDP}, for $i\in A$ and $A\in \mathcal{A}_\tau$, there exists $\mathcal{RV}_A^{\Pi^{(j)}}(\bar{x}, \bar{X}^{(j)})$ satisfying $(\epsilon_i^{(j)}, \delta_i^{(j)})$-DP. By Lemma \ref{lemma:RV_comb}, $(\mathcal{RV}_A^{\Pi^{(j)}}(\bar{x}, \bar{X}^{(j)}))_{j=1}^m$ is a refined view for $A\in \mathcal{A}_\tau$ in $\Pi$. By the composition theorem of DP, $(\mathcal{RV}_A^{\Pi^{(j)}}(\bar{x}, \bar{X}^{(j)}))_{j=1}^m$ is $(\Sigma_{j=1}^m \epsilon_i^{(j)}, \Sigma_{j=1}^m \delta_i^{(j)})$-differentially private. Thus $\Pi$ is perfectly $(\tau,n,\mathcal{E})$-TPMDP.
        By Lemma \ref{lemma:RV_comb}, we can similarly prove Theorem \ref{thm:m_comp_thm} for the cases of statistically and computationally TPMDP.
    \end{proof}
    
    For the $m$-fold composition of $(\tau, n, \mathcal{E})$-TPMDP mechanisms, we present an advanced composition theorem which allows the privacy parameters to decay more slowly.
    
    \begin{theorem}[Advanced Composition for TPMDP] \label{thm:m_A_comp}
        Let Assumption \ref{ass:comp_mech} hold and $\hat{\mathcal{E}} \triangleq ((\hat{\epsilon}_i, \hat{\delta}_i))_{i=1}^n$. Then for all $\delta_i > 0,\, i\in \{1,\hdots,n\}$, $\Pi$ is
        \begin{enumerate}
            \item perfectly $(\tau,n,\mathcal{E})$-TPMDP if $\Pi^{(j)}$ is perfectly $(\tau,n,\hat{\mathcal{E}})$-TPMDP for $j \in \{1,$ $\hdots,m\}$;
            \item statistically (computationally) $(\tau,n,\mathcal{E})$-TPMDP if $\Pi^{(j)}$ is statistically (computationally) $(\tau,n,\hat{\mathcal{E}})$-TPMDP for $j\in \{1,\hdots,m\}$ and $m$ is polynomial related to $\left| \bar{x} \right|$,
        \end{enumerate}
        where $\mathcal{E} = ((\epsilon_i, m\hat{\delta}_i + \delta_i))_{i=1}^n$ and for $i\in \{1,\hdots,n\}$,
        $$
        \epsilon_i = \sqrt{2m \ln{(1/\delta_i)}} \hat{\epsilon}_i + m\hat{\epsilon}_i (\exp{(\hat{\epsilon}_i)}-1).
        $$
    \end{theorem}
%}
